# Supplementary material for: Kohn-Sham potentials in exact density-functional theory at non-integer electron numbers
Source: arXiv:1407.2707 source file (2014-10-26)
Supplement: Supplementary file 1 [file KSPotential_Supp.pdf]

# Supplementary material for “Kohn-Sham potentials in exact density-functional theory at non-integer electron numbers”

This text contains supplementary material for “Kohn-Sham potentials in exact density-functional theory at non-integer electron numbers” [1].

## I. FITTING OF THE QMC DENSITY

| Atom | Cation               | Neutral              | Anion                |
|------|----------------------|----------------------|----------------------|
| Li   | $7.2800 \pm 0.00002$ | $7.4781 \pm 0.00006$ | $7.5007 \pm 0.00008$ |
| C    | $37.4259 \pm 0.0004$ | $37.8354 \pm 0.0005$ | $37.8795 \pm 0.0005$ |
| F    | $99.0772 \pm 0.0007$ | $99.7189 \pm 0.0007$ | $99.8443 \pm 0.0007$ |

TABLE I. Absolute ground-state DMC energies.

We fit the electron density of the atoms and ions to a function

$$n^M(r) = (1+r)^{g-1} \sum_{\kappa=1}^n \frac{a_0^\kappa + a_1^\kappa r^2}{b_0^\kappa + r^2} e^{-K^\kappa r}, \quad (1)$$

where  $K^1 = 2k$ ,  $K^{\kappa>1} > K^1$  and

$$k = \sqrt{-2\epsilon_h^M}, \quad g = \frac{Z+1-M}{k}. \quad (2)$$

This fitting function ensures that the density obeys the correct asymptotic behaviour [2]

$$\lim_{r \rightarrow \infty} \frac{\frac{1}{2} \nabla^2 \sqrt{n^M(r)}}{\sqrt{n^M(r)}} = -\frac{Z+1-M}{r} - \epsilon_h^M, \quad (3)$$

where  $-\epsilon_h = \frac{1}{2}k^2$  is the second and first ionisation potential, or electron affinity of atom A for ions  $A^+$ , A and  $A^-$  respectively.

Normalisation of  $n$  was carried out after fitting to the QMC data, to ensure that the electron number was preserved according to the appropriate abscissae and weights. QMC ground-state energies [reported in Table I] were used to calculate  $I$  and  $A$ . Values for the second ionisation potential came from the NIST database [3].

Parameters used for the fitting function (1) are shown in Appendix A and were found by minimising

$$\int_0^\infty [n^M(r) - n_{\text{QMC}}^M(r)]^2 (Zr + r^2) dr, \quad (4)$$

where  $n_{\text{QMC}}^M$  is calculated in diffusion Monte Carlo (DMC) with Jastrow full-valence complete-active-space wave functions fully optimized at the variational Monte Carlo level [4]. The local errors from the fitted functions are less than the statistical error of the QMC calculations in the inner region, while the outer region matches exactly the QMC affinity or ionisation potential (IP) or experimental second IP.

## II. ADDITIONAL MESH PLOTS

In the main text we illustrate the derivative discontinuity and other unusual features of the KS potential directly by plotting  $v_s^{Z+c}(r)$  as a function of radius  $r$  and excess electron number  $c = N - Z$ . By noting that the Hartree potential  $v_H^{Z+c}(r) = \int \frac{dr'}{|r-r'|} n^{Z+c}(r')$  must be piecewise continuous as a function of  $c$  (since  $n$  is piecewise continuous) and the external potential  $v_{\text{Ext}}(r)$  is independent of  $c$  we see that these features must manifest in  $v_{\text{xc}}^{Z+c}(r) = v_s^{Z+c}(r) - v_{\text{Ext}}(r) - v_H^{Z+c}(r)$ . We thus show, in Figure 1 plots of  $v_{\text{xc}}^{Z+c}(r)$  for the three species to highlight in greater detail some of its important features. We include also  $v_{\text{Hxc}}^{Z+c}(r)$  to show the total internal effective potential.

## III. APPROXIMATION TO $V_s^N$

In equation (16) of the text we propose an approximation

$$n^N(\mathbf{r}) v_s^N(\mathbf{r}) \approx (1-f) n^M(\mathbf{r}) [v_s^{M-}(\mathbf{r}) + \Delta^M] + f n^{M+1}(\mathbf{r}) v_s^{M+1-}(\mathbf{r}) \quad (5)$$

which relates the KS potential at fractional electron number  $N$  to its values at adjacent integers. In Figure 2 we show the potential at  $r=1, 2, 4$  and  $8$  for  $-1 < c \leq 1$ . It is clear, at least for these selected values of  $r$ , that the approximation is very good. To reduce numerical errors we use  $\Delta^M$  calculated numerically via  $\Delta^M = \int d\mathbf{r} n^M(\mathbf{r}) [v_s^{M+0.01}(\mathbf{r}) - v_s^M(\mathbf{r})] / M$  in all cases. For  $M = Z$  this gives results within 3 mhartree of the theoretical prediction  $I - A$ .

In Figure 3 we show mesh plots of the difference between the approximate and actual Kohn-Sham potentials. We note that there are numerical issues in the QMC density and in the Kohn-Sham inversion algorithm for  $r \rightarrow 0$  and  $r \rightarrow \infty$ . We suspect that some of the error in these regions is due to this numerical noise. This is exemplified by  $c \rightarrow -1$ , where the fit should become almost exact, but clearly shows significant numerical deviation in all cases, but especially Li.

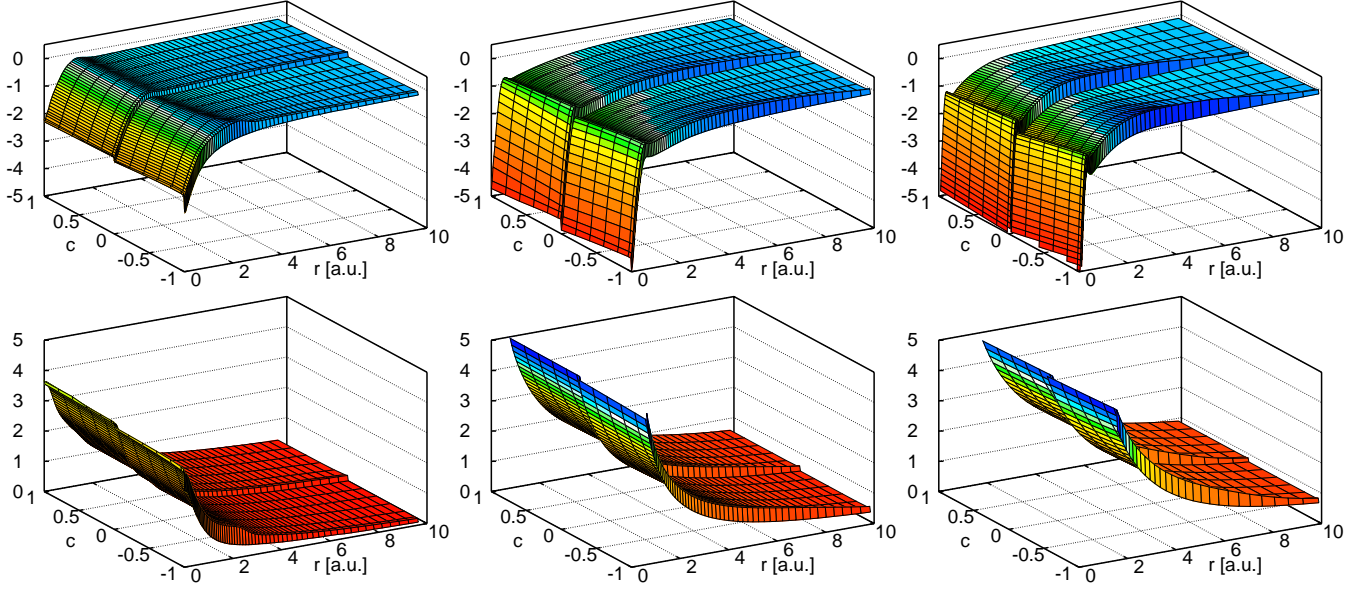

FIG. 1. xc potentials  $v_{xc}^{Z+c}(r)$  (top) and Hxc potentials  $v_{Hxc}^{Z+c}(r)$  (bottom) as a function of the radial distance  $r$  and the fractional excess electron number  $c = N - Z$  for Li (left), C (middle) and F (right).

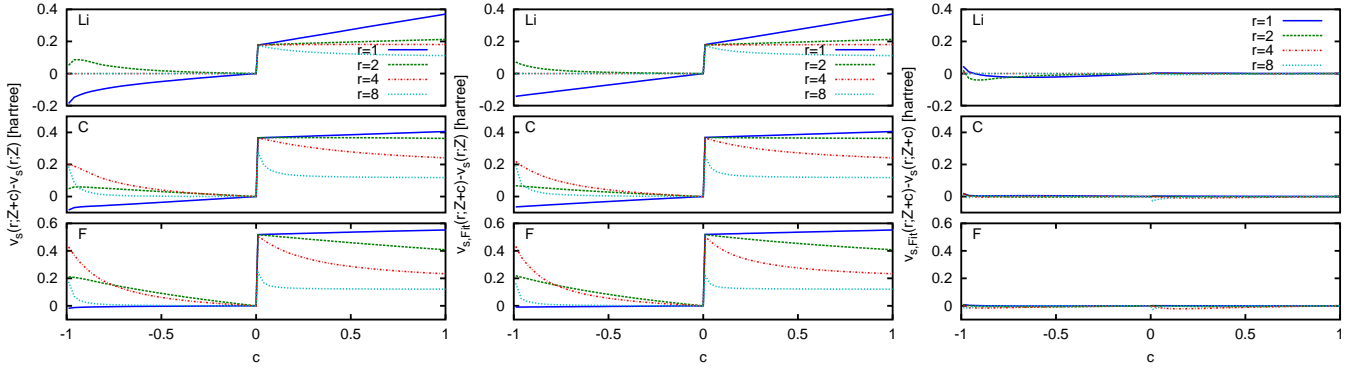

FIG. 2. Comparison of  $v_{s,approx}^{Z+c}(r)$  [from equation 16 of main text or (5) here] with  $v_s^{Z+c}(r)$  obtained from inversion. Left plot shows  $v_s^{Z+c}(r)$  (the same as Figure 2 in the paper), middle plot shows  $v_{s,approx}^{Z+c}(r)$ , and right column shows their difference.

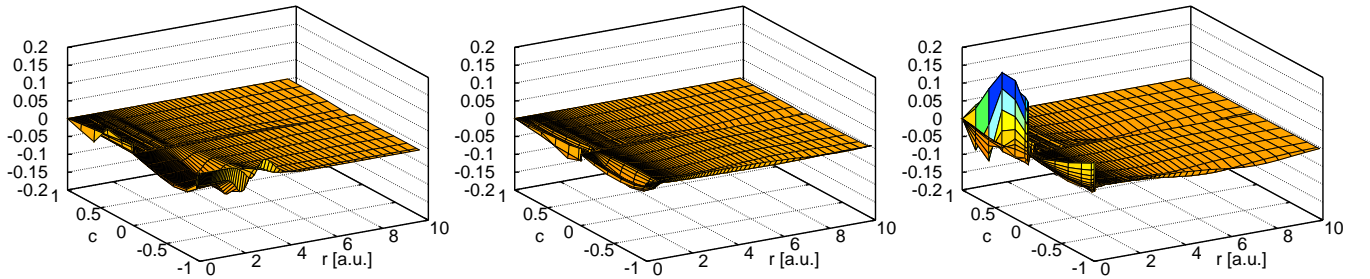

FIG. 3.  $v_{s,approx}^{Z+c}(r) - v_s^{Z+c}(r)$  for Li (left), C (middle) and F (right).

## Appendix A: Tables of fitting parameters

We provide here the parameters found by fitting the QMC density by the function given in Eq. 1.

### 1. Fitting parameters for Li ions.

|                               |         |         |        |        |
|-------------------------------|---------|---------|--------|--------|
| $\text{Li}^+ : g, \epsilon_h$ | 0.8488  | -2.7757 |        |        |
| $a_0^1, a_1^1, b_0^1, K^1$    | 0.3087  | 3.1382  | 0.1358 | 4.7123 |
| $a_0^2, a_1^2, b_0^2, K^2$    | 0.6979  | 5.4662  | 0.1078 | 4.8464 |
| $a_0^3, a_1^3, b_0^3, K^3$    | 0.6332  | 5.4767  | 0.1267 | 7.4059 |
| $\text{Li} : g, \epsilon_h$   | 1.5887  | -0.1981 |        |        |
| $a_0^1, a_1^1, b_0^1, K^1$    | 0.0000  | 0.0368  | 0.0000 | 1.2589 |
| $a_0^2, a_1^2, b_0^2, K^2$    | 0.0193  | -0.0663 | 0.0444 | 1.7221 |
| $a_0^3, a_1^3, b_0^3, K^3$    | 0.1859  | 6.1006  | 0.0649 | 5.6060 |
| $a_0^4, a_1^4, b_0^4, K^4$    | 1.0550  | 6.5475  | 0.1004 | 7.8585 |
| $\text{Li}^- : g, \epsilon_h$ | 0.0000  | -0.0227 |        |        |
| $a_0^1, a_1^1, b_0^1, K^1$    | -0.0000 | 0.3789  | 0.0000 | 0.4261 |
| $a_0^2, a_1^2, b_0^2, K^2$    | 0.6442  | -0.9637 | 0.1445 | 0.9173 |
| $a_0^3, a_1^3, b_0^3, K^3$    | 1.1321  | 13.2649 | 0.4060 | 4.6360 |
| $a_0^4, a_1^4, b_0^4, K^4$    | 0.6203  | 4.3880  | 0.0989 | 6.3464 |

### 2. Fitting parameters for C ions.

|                              |         |          |        |         |
|------------------------------|---------|----------|--------|---------|
| $\text{C}^+ : g, \epsilon_h$ | 1.4938  | -0.8963  |        |         |
| $a_0^1, a_1^1, b_0^1, K^1$   | 0.0038  | 0.5181   | 0.2303 | 2.6778  |
| $a_0^2, a_1^2, b_0^2, K^2$   | 0.2244  | 2.4283   | 0.1614 | 3.1094  |
| $a_0^3, a_1^3, b_0^3, K^3$   | 0.5551  | -5.9399  | 0.1294 | 4.6394  |
| $a_0^4, a_1^4, b_0^4, K^4$   | 2.0413  | -8.6682  | 0.1346 | 7.2725  |
| $a_0^5, a_1^5, b_0^5, K^5$   | 2.6932  | 26.9625  | 0.1116 | 11.5265 |
| $a_0^6, a_1^6, b_0^6, K^6$   | 6.8900  | 64.3988  | 0.0827 | 15.0396 |
| $\text{C} : g, \epsilon_h$   | 1.1050  | -0.4095  |        |         |
| $a_0^1, a_1^1, b_0^1, K^1$   | -0.0230 | 0.2497   | 0.0724 | 1.8100  |
| $a_0^2, a_1^2, b_0^2, K^2$   | 0.1274  | 1.9700   | 0.1031 | 2.3832  |
| $a_0^3, a_1^3, b_0^3, K^3$   | 0.5945  | -6.6976  | 0.1653 | 4.6147  |
| $a_0^4, a_1^4, b_0^4, K^4$   | 1.6819  | -8.1982  | 0.1044 | 7.0917  |
| $a_0^5, a_1^5, b_0^5, K^5$   | 3.0723  | 44.8323  | 0.1063 | 10.6443 |
| $a_0^6, a_1^6, b_0^6, K^6$   | 6.7880  | 56.5449  | 0.0873 | 14.3063 |
| $\text{C}^- : g, \epsilon_h$ | 0.0000  | -0.0441  |        |         |
| $a_0^1, a_1^1, b_0^1, K^1$   | 0.0162  | 0.1622   | 0.0099 | 0.5940  |
| $a_0^2, a_1^2, b_0^2, K^2$   | 0.4331  | 3.7392   | 0.0711 | 1.3221  |
| $a_0^3, a_1^3, b_0^3, K^3$   | 1.0876  | -17.8857 | 0.0919 | 3.6025  |
| $a_0^4, a_1^4, b_0^4, K^4$   | 2.2450  | 16.7874  | 0.1066 | 8.0515  |
| $a_0^5, a_1^5, b_0^5, K^5$   | 3.4417  | 38.3274  | 0.1032 | 10.0188 |
| $a_0^6, a_1^6, b_0^6, K^6$   | 5.5813  | 30.2854  | 0.1050 | 13.6394 |

### 3. Fitting parameters for F ions.

|                              |         |          |        |         |
|------------------------------|---------|----------|--------|---------|
| $\text{F}^+ : g, \epsilon_h$ | 1.2472  | -1.2857  |        |         |
| $a_0^1, a_1^1, b_0^1, K^1$   | -0.0483 | 1.8761   | 0.0117 | 3.2071  |
| $a_0^2, a_1^2, b_0^2, K^2$   | 0.4731  | 13.0823  | 0.0995 | 4.0844  |
| $a_0^3, a_1^3, b_0^3, K^3$   | 1.3455  | -12.2877 | 0.1049 | 7.2343  |
| $a_0^4, a_1^4, b_0^4, K^4$   | 6.5853  | -73.0653 | 0.0841 | 9.6721  |
| $a_0^5, a_1^5, b_0^5, K^5$   | 3.0913  | -69.6398 | 0.1197 | 15.0256 |
| $a_0^6, a_1^6, b_0^6, K^6$   | 29.5182 | 129.0790 | 0.0886 | 21.3125 |
| $\text{F} : g, \epsilon_h$   | 0.8827  | -0.6417  |        |         |
| $a_0^1, a_1^1, b_0^1, K^1$   | -0.0349 | 1.1718   | 0.0081 | 2.2657  |
| $a_0^2, a_1^2, b_0^2, K^2$   | 0.3246  | 13.2959  | 0.0862 | 3.4734  |
| $a_0^3, a_1^3, b_0^3, K^3$   | 1.8434  | -16.5528 | 0.0804 | 7.9333  |
| $a_0^4, a_1^4, b_0^4, K^4$   | 3.5155  | -37.2971 | 0.0817 | 8.4666  |
| $a_0^5, a_1^5, b_0^5, K^5$   | 6.9788  | -63.2687 | 0.0968 | 11.8701 |
| $a_0^6, a_1^6, b_0^6, K^6$   | 28.1609 | 24.6661  | 0.0905 | 21.1531 |
| $\text{F}^- : g, \epsilon_h$ | 0.0000  | -0.1254  |        |         |
| $a_0^1, a_1^1, b_0^1, K^1$   | 0.0122  | 0.7452   | 0.0021 | 1.0016  |
| $a_0^2, a_1^2, b_0^2, K^2$   | 0.6640  | 16.3921  | 0.0382 | 2.3493  |
| $a_0^3, a_1^3, b_0^3, K^3$   | 2.8523  | -51.0754 | 0.0994 | 6.9453  |
| $a_0^4, a_1^4, b_0^4, K^4$   | 2.3037  | -54.2370 | 0.1006 | 7.0417  |
| $a_0^5, a_1^5, b_0^5, K^5$   | 4.1322  | -31.2873 | 0.1015 | 10.8156 |
| $a_0^6, a_1^6, b_0^6, K^6$   | 7.6164  | -86.0300 | 0.0891 | 13.3094 |
| $a_0^7, a_1^7, b_0^7, K^7$   | 22.6386 | 30.0281  | 0.0924 | 20.6210 |

- 
- [1] T. Gould and J. Toulouse, ArXiv e-prints , 1407.2707 (2014).
  - [2] M. Levy, J. P. Perdew, and V. Sahni, Phys. Rev. A **30**, 2745 (1984).
  - [3] A. Kramida, Yu. Ralchenko, J. Reader, and NIST ASD Team, NIST Atomic Spectra Database (ver. 5.1), [Online]. Available: <http://physics.nist.gov/asd> [2014, March 8]. National Institute of Standards and Technology, Gaithersburg, MD. (2013).
  - [4] J. Toulouse, R. Assaraf, and C. J. Umrigar, J. Chem. Phys. **126**, 244112 (2007).
